# Supplementary material for: High sensitivity heat capacity measurements on Sr2RuO4 under uniaxial pressure
Source: arXiv:1906.07597 source file (2020-04-30)
Supplement: Supplementary file 1 [file Supplementary_Material_Li.pdf]

# High sensitivity heat capacity measurements on $Sr_2RuO_4$ under uniaxial pressure

## Supplemental Material

### A) Methods

High-quality single-crystal $Sr_2RuO_4$ samples were grown in a floating zone furnace (Canon Machinery) using techniques refined over many years to those described recently in Ref. 66. They were aligned using a bespoke Laue x-ray camera, and cut using a wire saw into thin bars with whose long axis aligned with the [100] direction of the crystal. For the best results these bars were polished using home-made apparatus based on diamond impregnated paper with a minimum grit size of 1 µm. The bar was then mounted within the jaws of the uniaxial pressure rig using Stycast 2850FT epoxy (Henkel Loctide). A resistive thin film resistor chip (State of the Art, Inc.) as heater and a calibrated Au-AuFe(0.07%) thermocouple are fixed to opposite sides of the sample using Dupont 6838 silver epoxy. Special care was taken when epoxying to the pressure cell to minimize tilt and ensure as homogeneous a strain field as possible.

The uniaxial pressure apparatus was mounted on a dilution refrigerator, with thermal coupling to the mixing chamber via a high purity silver wire. The data shown in the paper were acquired between 500 mK and 4.2 K, with operation above 1.5 K achieved by circulating a small fraction of the mixture. The thermocouple was spot-welded in-house and its calibration fixed by reference to that of a calibrated $RuO_2$ thermometer. The extremely low noise level of 20 pV/√Hz on the thermocouple readout was achieved by the combination of a low temperature transformer (CMR direct) mounted on the 1K pot of the dilution refrigerator, operating at a gain of 300, and an EG&G 7265 lock-in amplifier. A Keithley 6221 low-noise current source was used to drive the heater. The piezo electric actuators were driven at up to ± 400 V using a bespoke high-voltage amplifier.

In a setup of this kind, the significance of heat leaks to the environment is gauged by the lower cut-off frequency of set-up response curves such as those shown in Fig. 1b. By taking data at frequencies an order of magnitude higher than that lower cut-off, we ensure that the effect of such leaks makes a negligible contribution to our data.

### B) Heat capacity measurements in the temperature range between 0.5 and 4 K

In the main text, we have shown the heat capacity measurements between 1 and 4 K taken at a frequency of 3913 Hz. In Fig. S1 we present additional data at 2333 Hz in an extended temperature range down to 0.5 K. For each strain two data sets recorded in different temperature regions, from 0.5 K to 1.3 K and from 1 K to 4 K, have been combined. The data sets

of the two different measurement runs coincide in an excellent way in the overlap region. The increase in $T_c$ with strain is consistent with the result at $f_{exc}$ = 3913 Hz. Within our experimental resolution, we do not find any indication of an additional anomaly below the superconducting transition at any given strain.

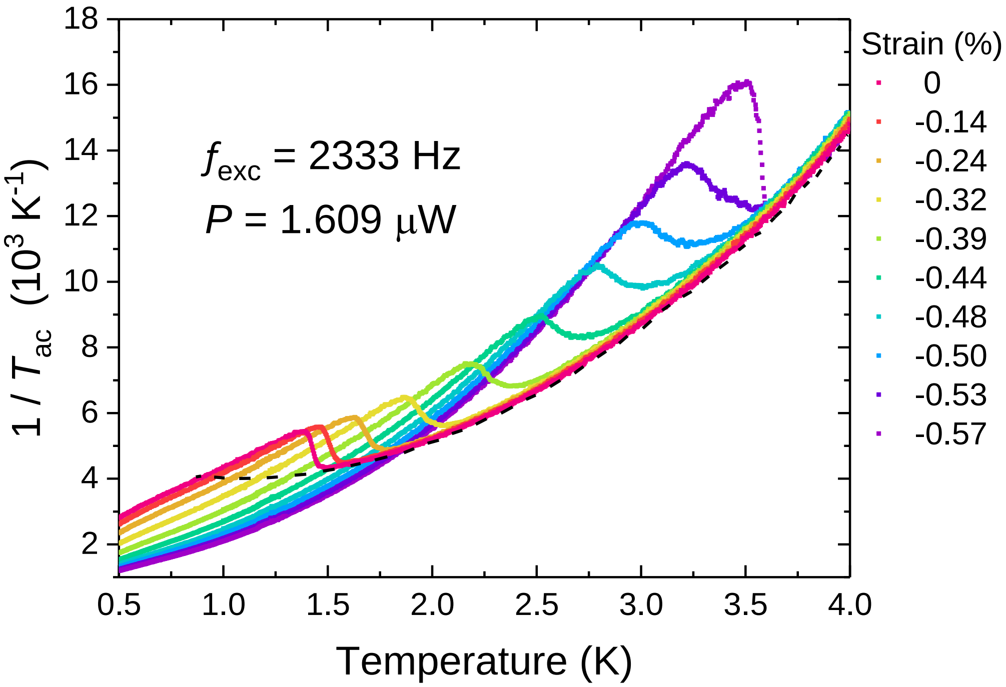


Fig. S1. Heat capacity measurements for sample S4 at $f_{exc}$ = 2333 Hz under various strains. $1/T_{ac}$ against temperature for different strains up to the peak in $T_c$. The dashed line is a heat capacity measurement at $\mu_0 H_{||c}$ = 0.1 T and $\varepsilon_{xx}$ = 0%.

**C) The relation between the heat capacity and the specific heat**

The conversion between the heat capacity and specific heat in a conventional setup is trivial, since the volume (or mass) of the sample is constant. In our measurements, the probed sample volume varies since the thermal diffusion length changes as a function of temperature. Therefore, it is nontrivial to convert our heat capacity data to specific heat. We start with an ideal case to demonstrate the relation between heat capacity and specific heat in case of our experimental setup.

Suppose that the heater contact is point-like and the sample is very narrow such that the heat flow is one-dimensional. The probed volume $V$ is equal to the cross-sectional area $A$ times twice, heat propagating on both sides, the diffusion length $l_{\mathrm{d}}$, which is a function of the frequency $\omega$, the volume specific heat $c_{\mathrm{v}}$ and the thermal conductivity $\kappa$.

$$l_{\mathrm{d}} = \sqrt{\frac{2\kappa(T)}{\omega c_{\mathrm{v}}(T)}} \quad \text{(S1)}$$

The experimentally obtained heat capacity $C_{\mathrm{ac}}$ can be expressed as follows:

$$C_{\mathrm{ac}} = c_{\mathrm{v}} \times V = c_{\mathrm{v}} \times A \times 2\sqrt{\frac{2\kappa}{\omega c_{\mathrm{v}}}} = \frac{2A}{\sqrt{\omega}}\sqrt{2\kappa(T)c_{\mathrm{v}}(T)} \quad \text{(S2)}$$

By inserting equation (S2) into equation (1), the temperature readout from the thermocouple is:

$$T_{\mathrm{ac}} = \frac{P * F(\omega)}{2A\sqrt{\omega} * \sqrt{2\kappa(T)c_{\mathrm{v}}(T)}} \quad \text{(S3)}$$

The excitation frequencies in our current measurements are not far away from the upper cut-off frequency, which describes the time scale for the heat propagating from the heater to the thermocouple, so the frequency response at the excitation frequencies $F(\omega) < 1$ and depends on temperature. Consequently, it is not possible to obtain the specific heat in the current sample configuration. However, we can normalize the data in the superconducting state by the normal state data to eliminate $F(\omega)$:

$$\frac{C_{\mathrm{ac}}^{\mathrm{s}}}{C_{\mathrm{ac}}^{\mathrm{n}}} = \frac{T_{\mathrm{ac}}^{\mathrm{n}}}{T_{\mathrm{ac}}^{\mathrm{s}}} = \sqrt{\frac{\kappa_{\mathrm{s}} c_{\mathrm{v}}^{\mathrm{s}}}{\kappa_{\mathrm{n}} c_{\mathrm{v}}^{\mathrm{n}}}} \quad \text{(S4)}$$

The validity of the Eqs. (S2) to (S4) is based on the above-mentioned assumptions that the heater contact is point-like and the heat flow is one-dimensional. In reality, both the sample width and the heater contact size are finite. This implies for the experimental setup to satisfy the assumptions of the examined model system, the exposed sample length ($l_{\mathrm{sample}}$) must be far longer than the heater length ($l_{\mathrm{h}}$) and the sample width ($w_{\mathrm{sample}}$), $l_{\mathrm{sample}} \gg l_{\mathrm{h}}, w_{\mathrm{sample}}$. For sample S4 we have $l_{\mathrm{sample}}(2\ \mathrm{mm}) > l_{\mathrm{h}}(0.5\ \mathrm{mm}), w_{\mathrm{sample}}(0.2\ \mathrm{mm})$. This shows that our current setup already is a good proof of principle, although, the described conditions are not perfectly met. Future designs will aim at $F(\omega) = 1$ and $l_{\mathrm{sample}} \gg l_{\mathrm{h}}, w_{\mathrm{sample}}$ to enable quantitative measurements of $c_{\mathrm{v}}(T)$ under strain.

**D) Experimental limits**

*Experimental limits on the detection of a potential second superconducting transition*

The signal-to-noise ratio determines one of the experimental limits on detecting a potential second superconducting transition in $Sr_2RuO_4$. The noise level remains almost the same for all strains; therefore, we used the heat capacity data at zero strain to analyze the experimental

resolution limit given by the noise of the thermometer readout. Fig. S2a shows the raw signal $V_{ac}$ of the thermocouple as function of temperature. The high sensitivity voltage readout was achieved by a transformer (300x amplification) mounted on the 1 K pot of the dilution refrigerator and using time constants of 20 and 50 s for 2333 and 3913 Hz, respectively. To determine the noise we fit a polynomial to the normal state data and subtracted it. Fig. S2b shows the result as function of temperature. The noise is temperature-independent and its standard deviation $\sigma$ is only 2.1 pV at the thermocouple.

Since 95% of data points fall within twice the standard deviation in a normal distribution, we use $4\sigma \approx 8.4\ \mathrm{pV}$ as the detection limit for a step size. The size of the signal at $T$ = 1.6 K is about 0.7 nV so the experimental limit on detecting a small jump in $\Delta c/c$ is $\Delta V_{\mathrm{ac}}/V_{\mathrm{ac}} = 8.4\ \mathrm{pV}\ /0.7\ \mathrm{nV} = 0.012$. The visible transition in the data has a jump size of $\Delta c/c \approx 0.3$. That implies that a potential second transition has to be more than $0.012/0.3 = 4\%$ of the size of the visible transition to be resolved. Therefore, the experimental limit on detecting the second transition is about 4% of the visible one for S4 with $f_{\mathrm{exc}}$ = 3913 Hz in the temperature region around 1.6 K.

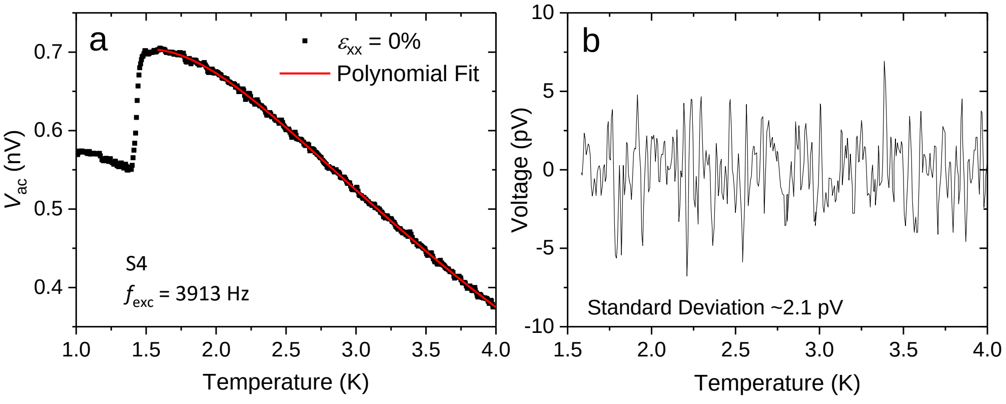


Fig. S2. Raw signal and noise. (a) The thermocouple voltage readout $V_{\mathrm{ac}}$ against temperature at zero strain for S4. The red line is a fit to the normal state data with a 5$^{\mathrm{th}}$ degree polynomial. (b) The difference between the measured signal $V_{\mathrm{ac}}$ and the fitted curve. The standard deviation is about 2.1 pV.

*The limit on determining the separation of two potential transitions*

It will be not possible to resolve two transitions if they are too close together. Therefore, in $Sr_2RuO_4$ the breadth of the visible transition determines the detection limit for the separation of two transitions. Fig. S3a and S3b show the first derivative of the measured $1/T_{\mathrm{ac}}(T)$ data with $f_{exc}$ = 3913 Hz at strains before and after the peak in $T_{\mathrm{c}}$ for S4, respectively. The full width at half maximum (FWHM) is used as a conservative criterion for the limit on determining the separation of two potential transitions. The results are shown in Fig. S3c. The FWHM increases from 50 mK at zero strain to 300 mK at $\varepsilon_{xx}$ = -0.53%.

*Strain inhomogeneity*

Strain inhomogeneity causes a distribution of $T_c$'s and leads to a rounded heat capacity anomaly. From the breadth of the transition, the size of the inhomogeneity can be estimated as follows:

$$\Delta T_{\mathrm{c}} \cong \frac{dT_{\mathrm{c}}(\varepsilon)}{d\varepsilon} \times \Delta\varepsilon = \frac{dT_{\mathrm{c}}(\varepsilon)}{d\varepsilon} \times \frac{\Delta\varepsilon}{\varepsilon} \times \varepsilon. \qquad \text{(S5)}$$

$\Delta T_{\mathrm{c,FWHM}}$ can be determined from the $d(1/T_{\mathrm{ac}})/dT$ curves as shown in Fig. S3 and, therefore,

$$\Delta T_{\mathrm{c,FWHM}} = \left|\frac{dT_{\mathrm{c}}(\varepsilon)}{d\varepsilon}\right| \times \frac{\Delta\varepsilon_{\mathrm{FWHM}}}{|\varepsilon|} \times |\varepsilon|. \qquad \text{(S6)}$$

The distribution in $T_c$, $\Delta T_{\mathrm{c,FWHM}}$, is related to the tangent slope on the $T_{\mathrm{c}}(\varepsilon)$ curve $|dT_{\mathrm{c}}(\varepsilon)/d\varepsilon|$, the strain inhomogeneity $\Delta\varepsilon_{\mathrm{FWHM}}/|\varepsilon|$ and the applied strain $|\varepsilon|$. It is inevitable to have a certain strain inhomogeneity in a sample and, therefore, the higher the applied strain, the wider the distribution in $T_c$. Note, the distribution is even larger when the applied strain goes beyond $\varepsilon_{\mathrm{peak\ in\ T_c}}$ because the tangent slope is steeper. The $T_{\mathrm{c}}(\varepsilon)$ curve determined by the midpoints of the leading edge of the transitions is used to simulate $\Delta T_{\mathrm{c,FWHM}}$ with different sizes of the inhomogeneity as shown in Fig. S3c. The values of $\Delta T_{\mathrm{c,FWHM}}$ near zero strain are different from the simulations because there is a finite transition width intrinsic to the sample. The distribution of $T_c$ scales with the tangent slope on $T_{\mathrm{c}}(\varepsilon)$. Hence, the inhomogeneity determined primarily by matching to the simulations around the peak in $T_c$ is approximately 8% in sample S4.

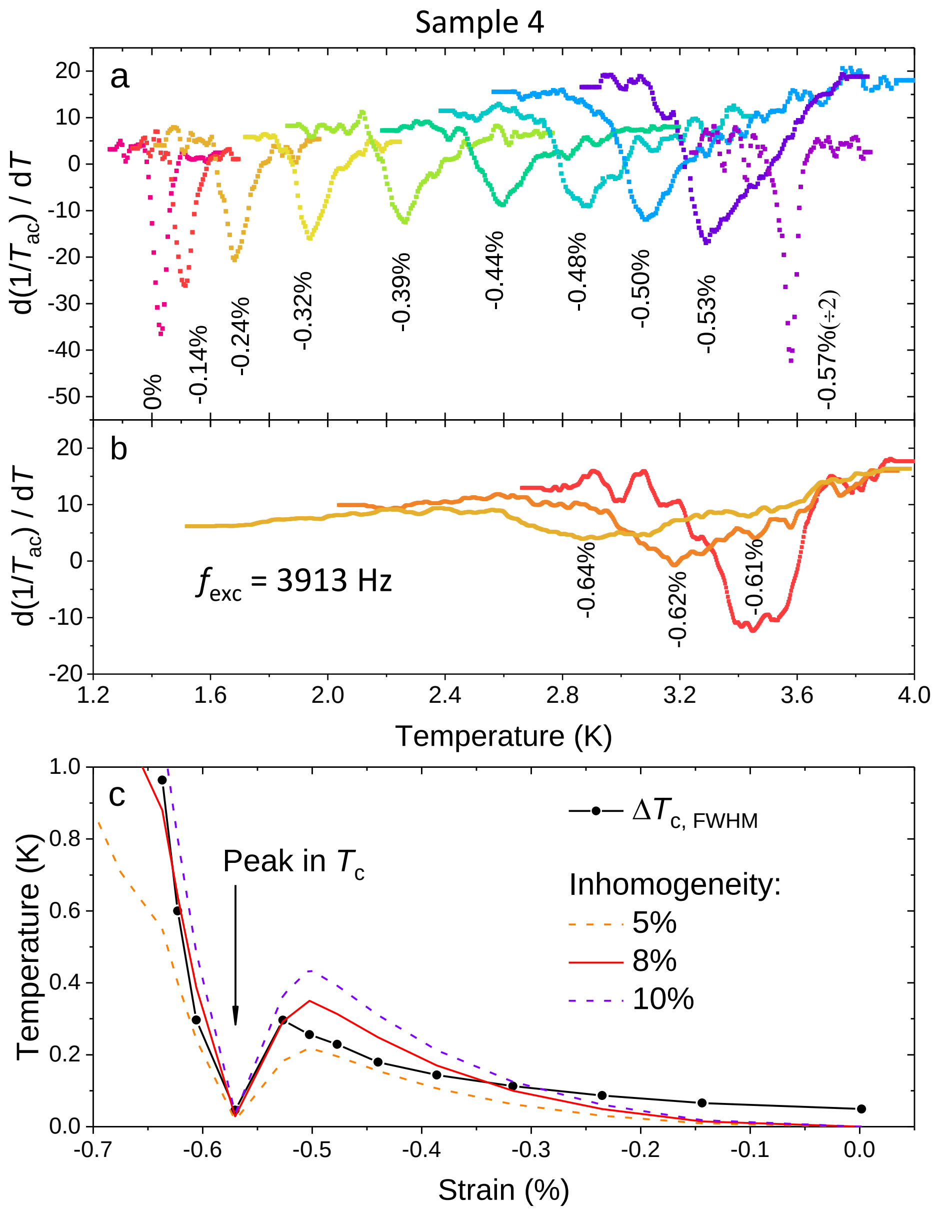


Fig. S3. Temperature resolution and strain inhomogeneity. The first derivative of $1/T_{ac}$ with respect to temperature for S4 at different strains (a), before the peak in $T_c$ and (b), after the peak. The curve at -0.57% in panel a is reduced by a factor of 2 for clarity. (c) The transition breadth against strain. The solid points are the FWHM derived from the results in (a) and (b). Three simulation curves (see text) with different strain inhomogeneities are shown for comparison. The arrow marks the position of the peak in $T_c$.

References:


[66] Bobowski, J. S. *et al.* Improved Single-Crystal Growth of $Sr_2RuO_4$. *Condens. Matter* **4**, 6 (2019).
